# Supplementary material for: Integrated ab initio modelling of atomic order and magnetic anisotropy for rare-earth-free magnet design: effects of alloying additions in $\mathrm{L}1_0$ FeNi
Source: arXiv:2401.02809 ancillary file (2024-11-29)
Supplement: Supplementary file 1 [file supplemental.pdf]

# Integrated *ab initio* modelling of atomic order and magnetic anisotropy for rare-earth-free magnet design: effects of alloying additions in $L1_0$ FeNi

## Supplemental Material

Christopher D. Woodgate,[1,*] Laura H. Lewis,[2,3] and Julie B. Staunton[1,†]

[1] *Department of Physics, University of Warwick, Coventry, CV4 7AL, United Kingdom*
[2] *Department of Chemical Engineering, Northeastern University, Boston, MA 02115, USA*
[3] *Department of Mechanical and Industrial Engineering, Northeastern University, Boston, MA 02115, USA*

This is the supplemental material accompanying the main text. Here we visualise eigenvalues of the chemical stability matrix for the considered systems, tabulate our fitted atom-atom interactions, and provide results from Monte Carlo simulations not included in the main text. The atom-atom interchange parameters are for the Bragg-Williams Hamiltonian, which takes the form

$$H = \frac{1}{2} \sum_{i\alpha;j\alpha'} V_{i\alpha;j\alpha'} \xi_{i\alpha} \xi_{j\alpha'}. \tag{1}$$

However, assuming interactions are isotropic, we can write $V^{(n)}_{\alpha\alpha'}$ to denote the interaction between species $\alpha$ and $\alpha'$ on coordination shell $n$. Then Eq. 1 takes the form

$$H = \frac{1}{2} \sum_{i} \sum_{n} \left( \sum_{j\in n(i)} \sum_{\alpha\alpha'} V^{(n)}_{\alpha\alpha'} \xi_{i\alpha} \xi_{j\alpha'} \right), \tag{2}$$

where $n(i)$ denotes the set of lattice sites which are $n$th nearest-neighbours to site $i$.

All Monte Carlo simulations are lattice-based. The simulation cell contained 2048 atoms, *i.e.* 8 fcc unit cells in each direction, with periodic boundary conditions applied. At each temperature $10^4$ MC steps per atom were performed and average quantities extracted. All results are averaged over an ensemble of 10 simulations.

* Christopher.Woodgate@warwick.ac.uk
† J.B.Staunton@warwick.ac.uk

## I. FeNi

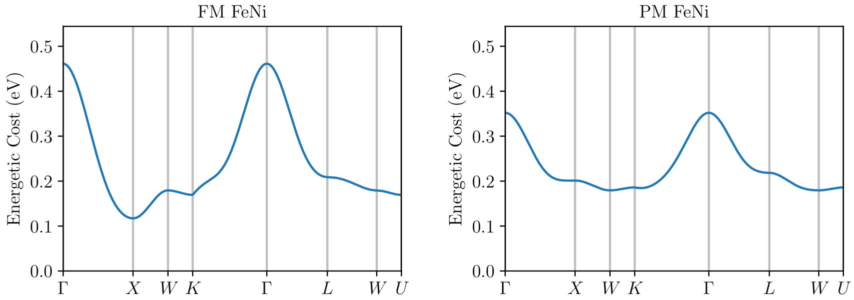


FIG. 1: Eigenvalues of the chemical stability matrix around the IBZ for FeNi modelled in its ferromagnetic (left) and paramagnetic (right) states. Both evaluated at $T = 1200$ K.

| Ferromagnetic | | | Paramagnetic | | |
|---|---|---|---|---|---|
| $V^{(1)}_{\alpha\alpha'}$ | Fe | Ni | $V^{(1)}_{\alpha\alpha'}$ | Fe | Ni |
| Fe | 7.50 | −7.50 | Fe | 4.14 | −4.14 |
| Ni | −7.50 | 7.50 | Ni | −4.14 | 4.14 |
| $V^{(2)}_{\alpha\alpha'}$ | Fe | Ni | $V^{(2)}_{\alpha\alpha'}$ | Fe | Ni |
| Fe | −0.24 | 0.24 | Fe | 0.86 | −0.86 |
| Ni | 0.24 | −0.24 | Ni | −0.86 | 0.86 |
| $V^{(3)}_{\alpha\alpha'}$ | Fe | Ni | $V^{(3)}_{\alpha\alpha'}$ | Fe | Ni |
| Fe | 1.63 | −1.63 | Fe | 0.28 | −0.28 |
| Ni | −1.63 | 1.63 | Ni | −0.28 | 0.28 |
| $V^{(4)}_{\alpha\alpha'}$ | Fe | Ni | $V^{(4)}_{\alpha\alpha'}$ | Fe | Ni |
| Fe | −0.26 | 0.26 | Fe | 0.75 | −0.75 |
| Ni | 0.26 | −0.26 | Ni | −0.75 | 0.75 |

TABLE I: Fitted atom-atom interactions for FeNi. All values in meV.

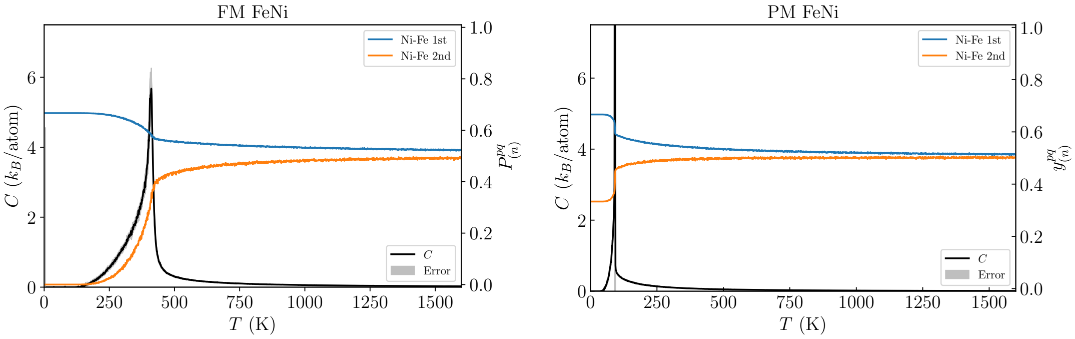


FIG. 2: Plots of the heat capacity and atomic order parameters for on-lattice Monte Carlo simulations of FeNi using our fitted atom-atom interactions obtained modelling either a ferromagnetic (left) or paramagnetic (right) state.

## II. $Fe_4Ni_3Pt$

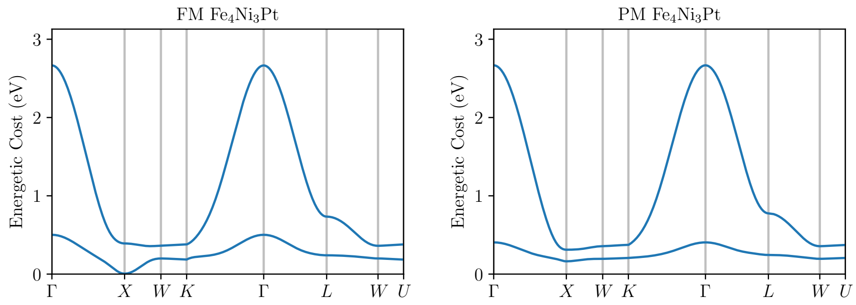


FIG. 3: Eigenvalues of the chemical stability matrix around the IBZ for $Fe_4Ni_3Pt$ modelled in its ferromagnetic (left) and paramagnetic (right) states. Both evaluated at $T = 1200$ K.

| Ferromagnetic | | | | Paramagnetic | | | |
|---|---|---|---|---|---|---|---|
| $V^{(1)}_{\alpha\alpha'}$ | Fe | Ni | Pt | $V^{(1)}_{\alpha\alpha'}$ | Fe | Ni | Pt |
| Fe | 11.81 | −4.63 | −33.36 | Fe | 6.87 | −1.42 | −23.40 |
| Ni | −4.63 | 9.78 | −10.83 | Ni | −1.42 | 9.93 | −24.38 |
| Pt | −33.36 | −10.83 | 165.91 | Pt | −23.40 | −24.38 | 168.29 |
| $V^{(2)}_{\alpha\alpha'}$ | Fe | Ni | Pt | $V^{(2)}_{\alpha\alpha'}$ | Fe | Ni | Pt |
| Fe | −1.82 | −0.16 | 7.75 | Fe | −1.55 | −0.19 | 6.83 |
| Ni | −0.16 | 4.41 | −12.61 | Ni | −0.19 | 3.92 | −11.10 |
| Pt | 7.75 | −12.61 | 6.82 | Pt | 6.83 | −11.10 | 6.11 |
| $V^{(3)}_{\alpha\alpha'}$ | Fe | Ni | Pt | $V^{(3)}_{\alpha\alpha'}$ | Fe | Ni | Pt |
| Fe | 2.45 | −1.53 | −5.21 | Fe | 0.74 | −0.28 | −2.17 |
| Ni | −1.53 | 0.47 | 4.70 | Ni | −0.28 | −0.22 | 1.76 |
| Pt | −5.21 | 4.70 | 6.73 | Pt | −2.17 | 1.76 | 3.40 |
| $V^{(4)}_{\alpha\alpha'}$ | Fe | Ni | Pt | $V^{(4)}_{\alpha\alpha'}$ | Fe | Ni | Pt |
| Fe | 0.25 | −0.56 | 0.67 | Fe | 1.18 | −0.98 | −1.76 |
| Ni | −0.56 | 0.32 | 1.27 | Ni | −0.98 | −0.07 | 4.16 |
| Pt | 0.67 | 1.27 | −6.49 | Pt | −1.76 | 4.16 | −5.53 |

TABLE II: Fitted atom-atom interactions for $Fe_4Ni_3Pt$. All values in meV.

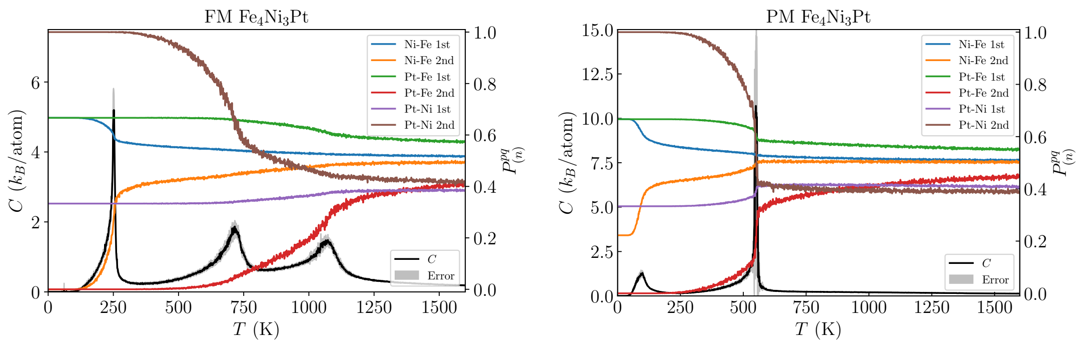


FIG. 4: Plots of the heat capacity and atomic order parameters for Monte Carlo simulations of $Fe_4Ni_3Pt$ using our fitted atom-atom interactions obtained modelling either a ferromagnetic (left) or paramagnetic (right) state.

## III. $Fe_4Ni_3Al$

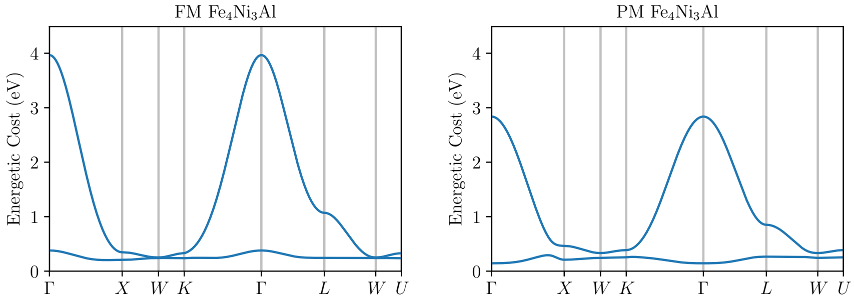


FIG. 5: Eigenvalues of the chemical stability matrix around the IBZ for $Fe_4Ni_3Al$ modelled in its ferromagnetic (left) and paramagnetic (right) states. Both evaluated at $T = 1200$ K.

| Ferromagnetic | | | | Paramagnetic | | | |
|---|---|---|---|---|---|---|---|
| $V^{(1)}_{\alpha\alpha'}$ | Fe | Ni | Al | $V^{(1)}_{\alpha\alpha'}$ | Fe | Ni | Al |
| Fe | 4.94 | 2.41 | −26.96 | Fe | −4.85 | 5.82 | 1.92 |
| Ni | 2.41 | 11.38 | −43.77 | Ni | 5.82 | 11.16 | −57.32 |
| Al | −26.96 | −43.77 | 239.15 | Al | 1.92 | −57.32 | 166.07 |
| $V^{(2)}_{\alpha\alpha'}$ | Fe | Ni | Al | $V^{(2)}_{\alpha\alpha'}$ | Fe | Ni | Al |
| Fe | −0.23 | 0.04 | 0.81 | Fe | 0.96 | −1.42 | 0.46 |
| Ni | 0.04 | 2.10 | −6.43 | Ni | −1.42 | 3.01 | −3.38 |
| Al | 0.81 | −6.43 | 16.06 | Al | 0.46 | −3.38 | 8.41 |
| $V^{(3)}_{\alpha\alpha'}$ | Fe | Ni | Al | $V^{(3)}_{\alpha\alpha'}$ | Fe | Ni | Al |
| Fe | 1.59 | −1.15 | −2.88 | Fe | −0.56 | 0.18 | 1.72 |
| Ni | −1.15 | 1.32 | 0.65 | Ni | 0.18 | 0.28 | −1.56 |
| Al | −2.88 | 0.65 | 9.57 | Al | 1.72 | −1.56 | −2.21 |
| $V^{(4)}_{\alpha\alpha'}$ | Fe | Ni | Al | $V^{(4)}_{\alpha\alpha'}$ | Fe | Ni | Al |
| Fe | 0.72 | 0.14 | −3.30 | Fe | 1.50 | −1.11 | −2.69 |
| Ni | 0.14 | −0.27 | 0.26 | Ni | −1.11 | 0.32 | 3.52 |
| Al | −3.30 | 0.26 | 12.41 | Al | −2.69 | 3.52 | 0.15 |

TABLE III: Fitted atom-atom interactions for $Fe_4Ni_3Al$. All values in meV.

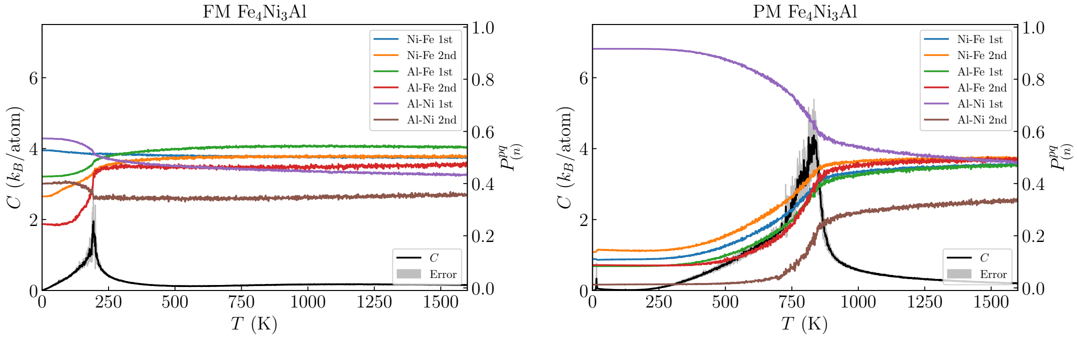


FIG. 6: Plots of the heat capacity and atomic order parameters for Monte Carlo simulations of $Fe_4Ni_3Al$ using our fitted atom-atom interactions obtained modelling either a ferromagnetic (left) or paramagnetic (right) state.

## IV. $Fe_4Ni_3Cr$

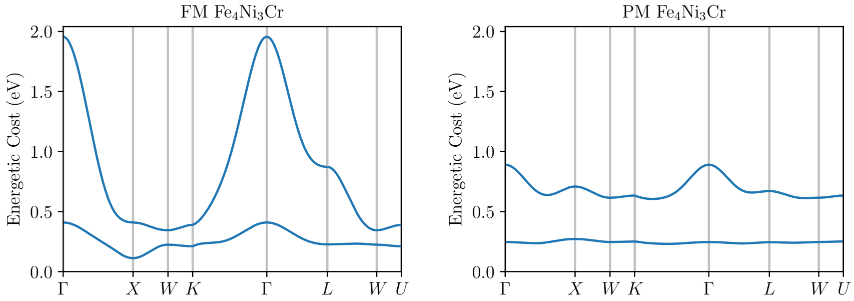


FIG. 7: Eigenvalues of the chemical stability matrix around the IBZ for $Fe_4Ni_3Cr$ modelled in its ferromagnetic (left) and paramagnetic (right) states. Both evaluated at $T = 1200$ K.

| Ferromagnetic | | | | Paramagnetic | | | |
|---|---|---|---|---|---|---|---|
| $V^{(1)}_{\alpha\alpha'}$ | Fe | Ni | Cr | $V^{(1)}_{\alpha\alpha'}$ | Fe | Ni | Cr |
| Fe | 7.62 | −2.84 | −21.96 | Fe | −0.48 | 0.81 | −0.50 |
| Ni | −2.84 | 5.28 | −4.49 | Ni | 0.81 | −0.34 | −2.25 |
| Cr | −21.96 | −4.49 | 101.28 | Cr | −0.50 | −2.25 | 8.84 |
| $V^{(2)}_{\alpha\alpha'}$ | Fe | Ni | Cr | $V^{(2)}_{\alpha\alpha'}$ | Fe | Ni | Cr |
| Fe | −0.61 | −1.07 | 5.64 | Fe | 0.41 | −1.09 | 1.64 |
| Ni | −1.07 | 2.33 | −2.70 | Ni | −1.09 | 2.82 | −4.17 |
| Cr | 5.64 | −2.70 | −14.47 | Cr | 1.64 | −4.17 | 6.04 |
| $V^{(3)}_{\alpha\alpha'}$ | Fe | Ni | Cr | $V^{(3)}_{\alpha\alpha'}$ | Fe | Ni | Cr |
| Fe | 1.78 | −1.18 | −3.57 | Fe | −0.05 | 0.07 | 0.01 |
| Ni | −1.18 | 0.99 | 1.77 | Ni | 0.07 | 0.11 | −0.61 |
| Cr | −3.57 | 1.77 | 8.97 | Cr | 0.01 | −0.61 | 1.79 |
| $V^{(4)}_{\alpha\alpha'}$ | Fe | Ni | Cr | $V^{(4)}_{\alpha\alpha'}$ | Fe | Ni | Cr |
| Fe | −0.25 | 0.54 | −0.61 | Fe | 0.20 | −0.62 | 1.07 |
| Ni | 0.54 | 0.23 | −2.85 | Ni | −0.62 | 1.88 | −3.21 |
| Cr | −0.61 | −2.85 | 11.01 | Cr | 1.07 | −3.21 | 5.41 |

TABLE IV: Fitted atom-atom interactions for $Fe_4Ni_3Cr$. All values in meV.

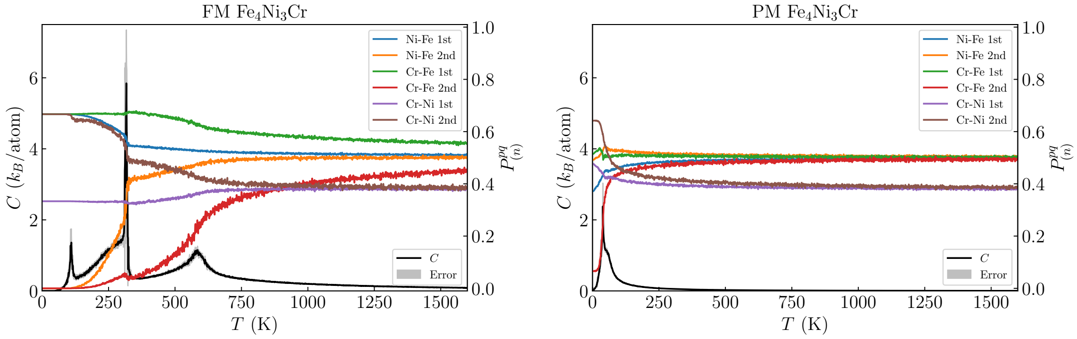


FIG. 8: Plots of the heat capacity and atomic order parameters for Monte Carlo simulations of $Fe_4Ni_3Cr$ using our fitted atom-atom interactions obtained modelling either a ferromagnetic (left) or paramagnetic (right) state.

## V. $Fe_4Ni_3Co$

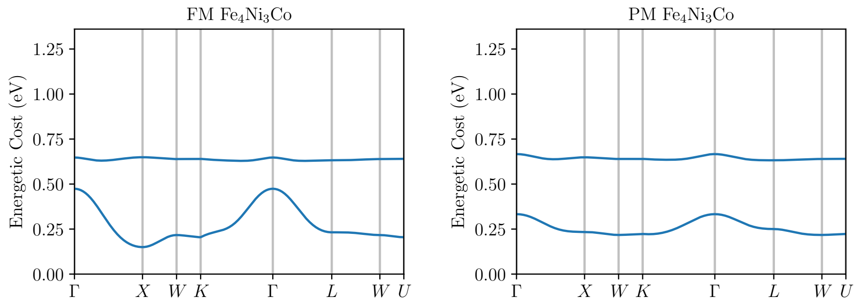


FIG. 9: Eigenvalues of the chemical stability matrix around the IBZ for $Fe_4Ni_3Co$ modelled in its ferromagnetic (left) and paramagnetic (right) states. Both evaluated at $T = 1200$ K.

| Ferromagnetic | | | | Paramagnetic | | | |
|---|---|---|---|---|---|---|---|
| $V^{(1)}_{\alpha\alpha'}$ | Fe | Ni | Co | $V^{(1)}_{\alpha\alpha'}$ | Fe | Ni | Co |
| Fe | 6.57 | −7.36 | −4.21 | Fe | 4.06 | −3.34 | −6.21 |
| Ni | −7.36 | 7.95 | 5.57 | Ni | −3.34 | 1.93 | 7.63 |
| Co | −4.21 | 5.57 | 0.14 | Co | −6.21 | 7.63 | 1.91 |
| $V^{(2)}_{\alpha\alpha'}$ | Fe | Ni | Co | $V^{(2)}_{\alpha\alpha'}$ | Fe | Ni | Co |
| Fe | 0.19 | −0.23 | −0.07 | Fe | 0.69 | −0.96 | 0.10 |
| Ni | −0.23 | 0.37 | −0.20 | Ni | −0.96 | 1.37 | −0.30 |
| Co | −0.07 | −0.20 | 0.88 | Co | 0.10 | −0.30 | 0.51 |
| $V^{(3)}_{\alpha\alpha'}$ | Fe | Ni | Co | $V^{(3)}_{\alpha\alpha'}$ | Fe | Ni | Co |
| Fe | 1.36 | −1.66 | −0.45 | Fe | 0.34 | −0.25 | −0.60 |
| Ni | −1.66 | 2.01 | 0.63 | Ni | −0.25 | 0.08 | 0.78 |
| Co | −0.45 | 0.63 | −0.08 | Co | −0.60 | 0.78 | 0.07 |
| $V^{(4)}_{\alpha\alpha'}$ | Fe | Ni | Co | $V^{(4)}_{\alpha\alpha'}$ | Fe | Ni | Co |
| Fe | −0.34 | 0.46 | −0.03 | Fe | 0.44 | −0.72 | 0.43 |
| Ni | 0.46 | −0.60 | −0.05 | Ni | −0.72 | 1.12 | −0.48 |
| Co | −0.03 | −0.05 | 0.29 | Co | 0.43 | −0.48 | −0.27 |

TABLE V: Fitted atom-atom interactions for $Fe_4Ni_3Co$. All values in meV.

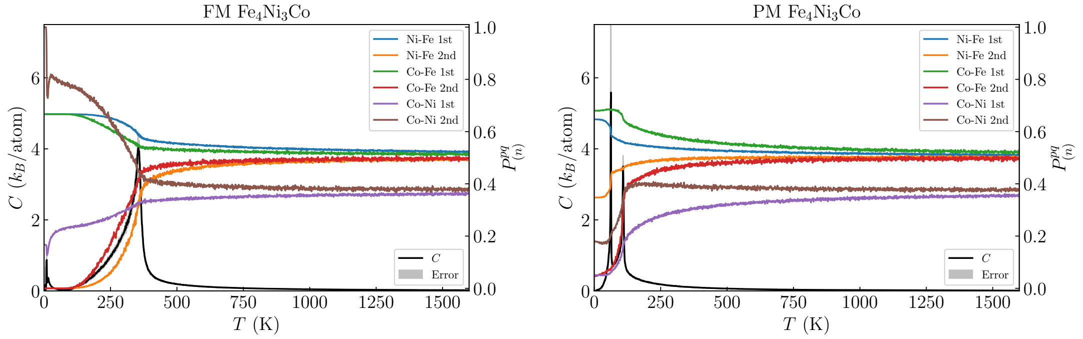


FIG. 10: Plots of the heat capacity and atomic order parameters for Monte Carlo simulations of $Fe_4Ni_3Co$ using our fitted atom-atom interactions obtained modelling either a ferromagnetic (left) or paramagnetic (right) state.

## VI. $Fe_4Ni_3Mo$

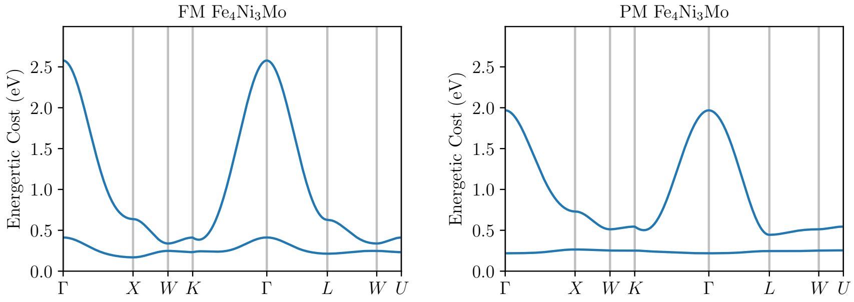


FIG. 11: Eigenvalues of the chemical stability matrix around the IBZ for $Fe_4Ni_3Mo$ modelled in its ferromagnetic (left) and paramagnetic (right) states. Both evaluated at $T = 1200$ K.

| Ferromagnetic | | | | Paramagnetic | | | |
|---|---|---|---|---|---|---|---|
| $V^{(1)}_{\alpha\alpha'}$ | Fe | Ni | Mo | $V^{(1)}_{\alpha\alpha'}$ | Fe | Ni | Mo |
| Fe | 4.76 | −0.38 | −17.91 | Fe | −1.05 | 2.55 | −3.51 |
| Ni | −0.38 | 8.22 | −23.13 | Ni | 2.55 | 4.94 | −25.26 |
| Mo | −17.91 | −23.13 | 141.04 | Mo | −3.51 | −25.26 | 90.71 |
| $V^{(2)}_{\alpha\alpha'}$ | Fe | Ni | Mo | $V^{(2)}_{\alpha\alpha'}$ | Fe | Ni | Mo |
| Fe | −0.10 | −0.54 | 2.04 | Fe | −0.12 | 0.22 | −0.20 |
| Ni | −0.54 | 6.32 | −16.80 | Ni | 0.22 | 5.37 | −17.19 |
| Mo | 2.04 | −16.80 | 42.25 | Mo | −0.20 | −17.19 | 52.93 |
| $V^{(3)}_{\alpha\alpha'}$ | Fe | Ni | Mo | $V^{(3)}_{\alpha\alpha'}$ | Fe | Ni | Mo |
| Fe | 1.71 | −1.62 | −1.99 | Fe | −0.05 | −0.23 | 0.89 |
| Ni | −1.62 | 1.32 | 2.51 | Ni | −0.23 | 0.26 | 0.14 |
| Mo | −1.99 | 2.51 | 0.46 | Mo | 0.89 | 0.14 | −4.00 |
| $V^{(4)}_{\alpha\alpha'}$ | Fe | Ni | Mo | $V^{(4)}_{\alpha\alpha'}$ | Fe | Ni | Mo |
| Fe | −0.25 | 0.43 | −0.28 | Fe | 0.14 | −0.59 | 1.23 |
| Ni | 0.43 | 0.13 | −2.11 | Ni | −0.59 | 1.01 | −0.68 |
| Mo | −0.28 | −2.11 | 7.46 | Mo | 1.23 | −0.68 | −2.90 |

TABLE VI: Fitted atom-atom interactions for $Fe_4Ni_3Mo$. All values in meV.

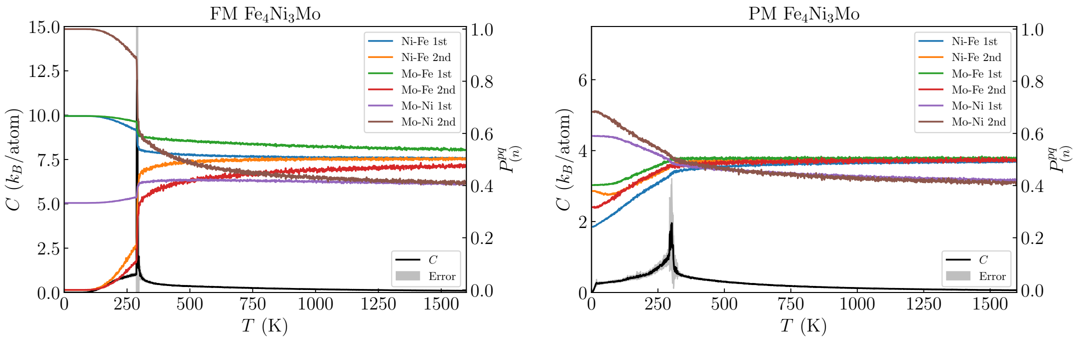


FIG. 12: Plots of the heat capacity and atomic order parameters for Monte Carlo simulations of $Fe_4Ni_3Mo$ using our fitted atom-atom interactions obtained modelling either a ferromagnetic (left) or paramagnetic (right) state.

## VII. $Fe_4Ni_3Pd$

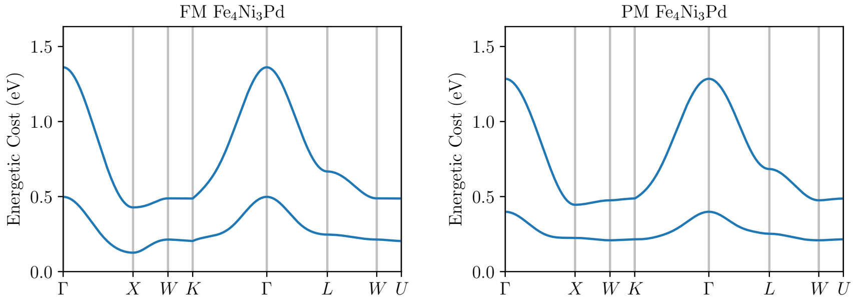


FIG. 13: Eigenvalues of the chemical stability matrix around the IBZ for $Fe_4Ni_3Pd$ modelled in its ferromagnetic (left) and paramagnetic (right) states. Both evaluated at $T = 1200$ K.

| Ferromagnetic | | | | Paramagnetic | | | |
|---|---|---|---|---|---|---|---|
| $V^{(1)}_{\alpha\alpha'}$ | Fe | Ni | Pd | $V^{(1)}_{\alpha\alpha'}$ | Fe | Ni | Pd |
| Fe | 7.25 | −6.01 | −10.98 | Fe | 3.60 | −3.63 | −3.52 |
| Ni | −6.01 | 10.06 | −6.15 | Ni | −3.63 | 9.42 | −13.92 |
| Pd | −10.98 | −6.15 | 62.37 | Pd | −3.52 | −13.92 | 56.39 |
| $V^{(2)}_{\alpha\alpha'}$ | Fe | Ni | Pd | $V^{(2)}_{\alpha\alpha'}$ | Fe | Ni | Pd |
| Fe | −1.34 | 0.09 | 5.10 | Fe | −0.65 | −0.55 | 4.30 |
| Ni | 0.09 | 1.63 | −5.27 | Ni | −0.55 | 2.20 | −4.46 |
| Pd | 5.10 | −5.27 | −4.59 | Pd | 4.30 | −4.46 | −3.80 |
| $V^{(3)}_{\alpha\alpha'}$ | Fe | Ni | Pd | $V^{(3)}_{\alpha\alpha'}$ | Fe | Ni | Pd |
| Fe | 2.11 | −1.64 | −3.52 | Fe | 0.54 | −0.33 | −1.17 |
| Ni | −1.64 | 1.14 | 3.16 | Ni | −0.33 | 0.07 | 1.13 |
| Pd | −3.52 | 3.16 | 4.57 | Pd | −1.17 | 1.13 | 1.29 |
| $V^{(4)}_{\alpha\alpha'}$ | Fe | Ni | Pd | $V^{(4)}_{\alpha\alpha'}$ | Fe | Ni | Pd |
| Fe | 0.07 | −0.11 | 0.05 | Fe | 1.02 | −0.74 | −1.86 |
| Ni | −0.11 | −0.10 | 0.71 | Ni | −0.74 | 0.18 | 2.46 |
| Pd | 0.05 | 0.71 | −2.33 | Pd | −1.86 | 2.46 | 0.05 |

TABLE VII: Fitted atom-atom interactions for $Fe_4Ni_3Pd$. All values in meV.

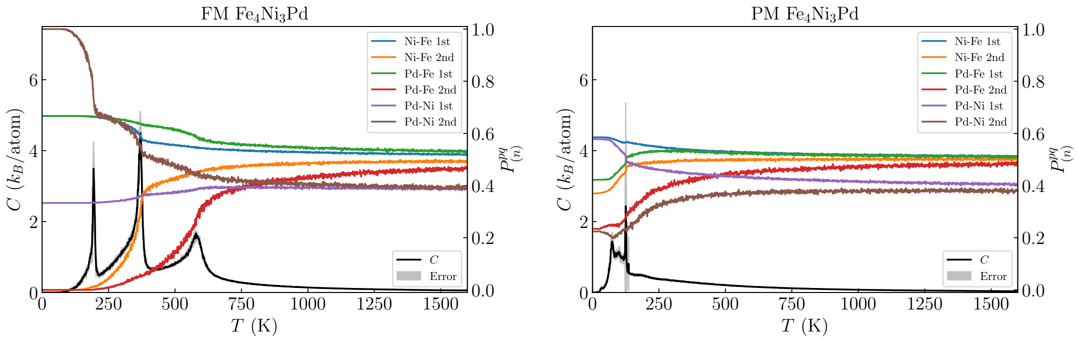


FIG. 14: Plots of the heat capacity and atomic order parameters for Monte Carlo simulations of $Fe_4Ni_3Pd$ using our fitted atom-atom interactions obtained modelling either a ferromagnetic (left) or paramagnetic (right) state.
